# Supplementary material for: A Large-Scale 3D Face Mesh Video Dataset via Neural Re-parameterized Optimization
Source: arXiv:2310.03205 source file (2023-10-06)
Supplement: Supplementary file 2 [file supp_grad_viz.tex]

\begin{figure}
    \centering
    % \vspace{6mm}
    \includegraphics[width=1\linewidth]{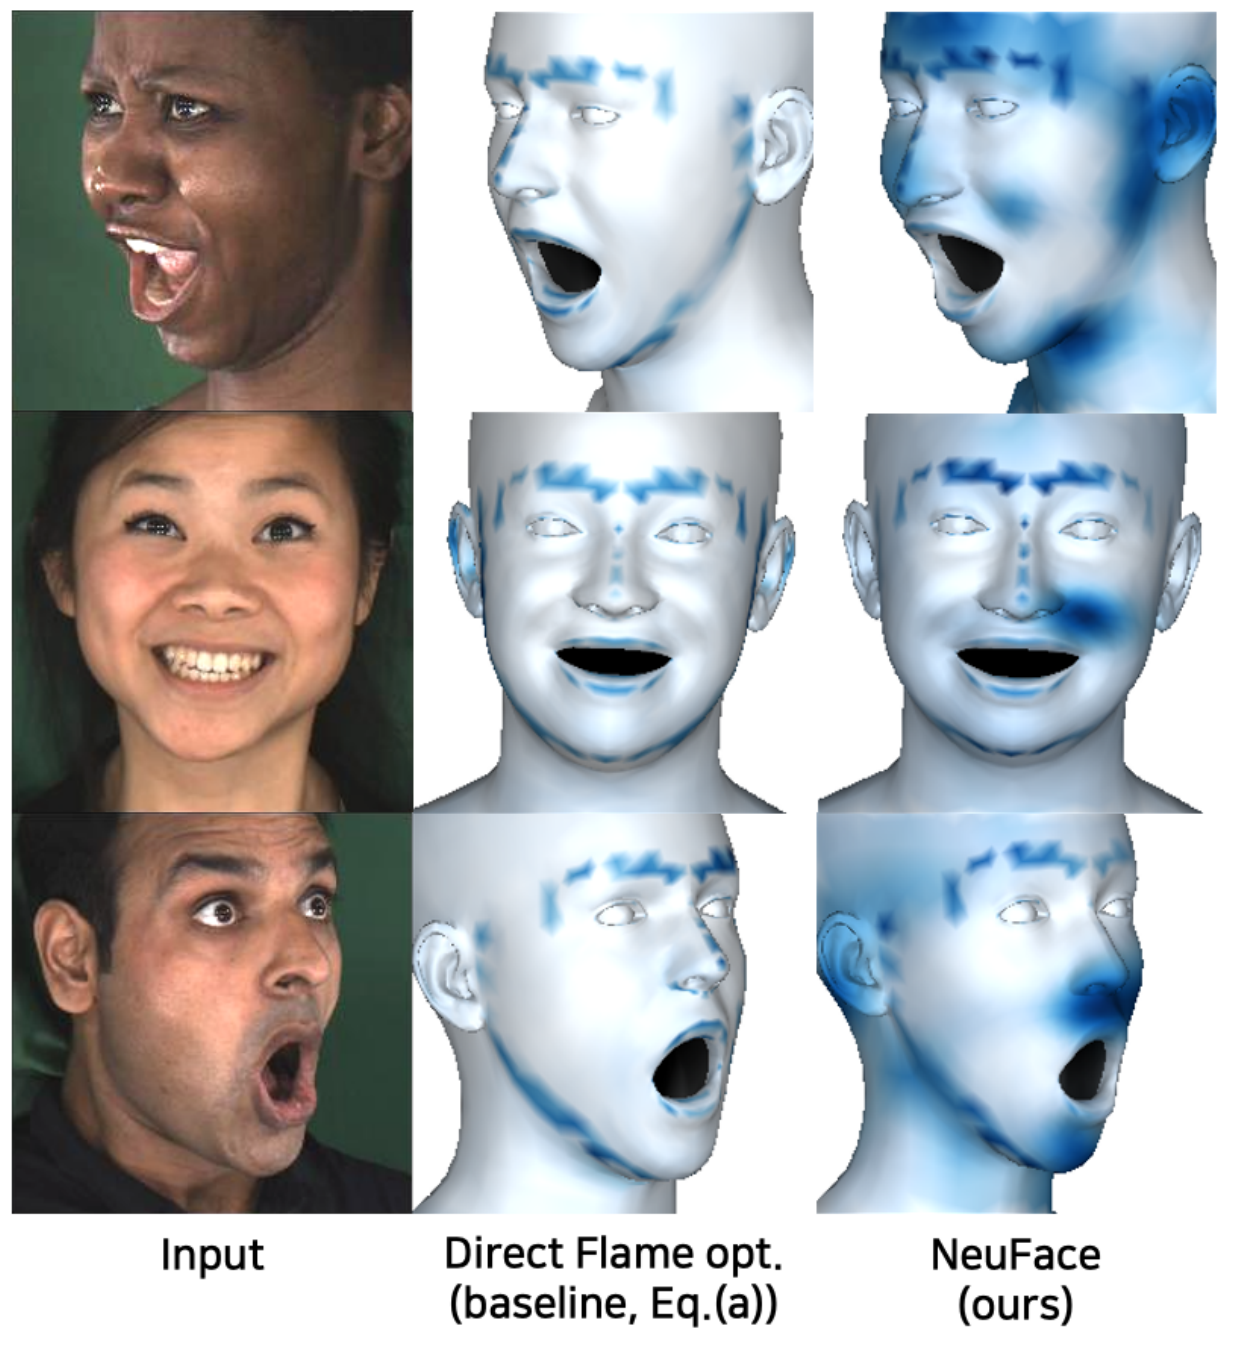}
    %\vspace{-1.5mm}
    \caption{\textbf{Data-dependent gradient of NeuFace.} While the baseline optimization produces similar gradient patterns over different 
    % input
    identities or expressions, NeuFace optimization produces diverse gradients dependent on input images 
    which helps capture
    % that help to 
    % capture 
    the expressive facial details. From white to blue, the absolute magnitude of the gradient becomes larger.
    % We compute single step mesh update gradients from iteration $t{=}0{\rightarrow}t{=}1$, thus all the meshes visualized are the same initialization from the pre-trained DECA.}
    }
    %\vspace{-3mm}
    \label{fig:supp_grad}
\end{figure}
