# Supplementary material for: A Large-Scale 3D Face Mesh Video Dataset via Neural Re-parameterized Optimization
Source: arXiv:2310.03205 source file (2023-10-06)
Supplement: Supplementary file 3 [file supp_voca_fig.tex]

\begin{figure}
    \centering
    \includegraphics[width=1\linewidth]{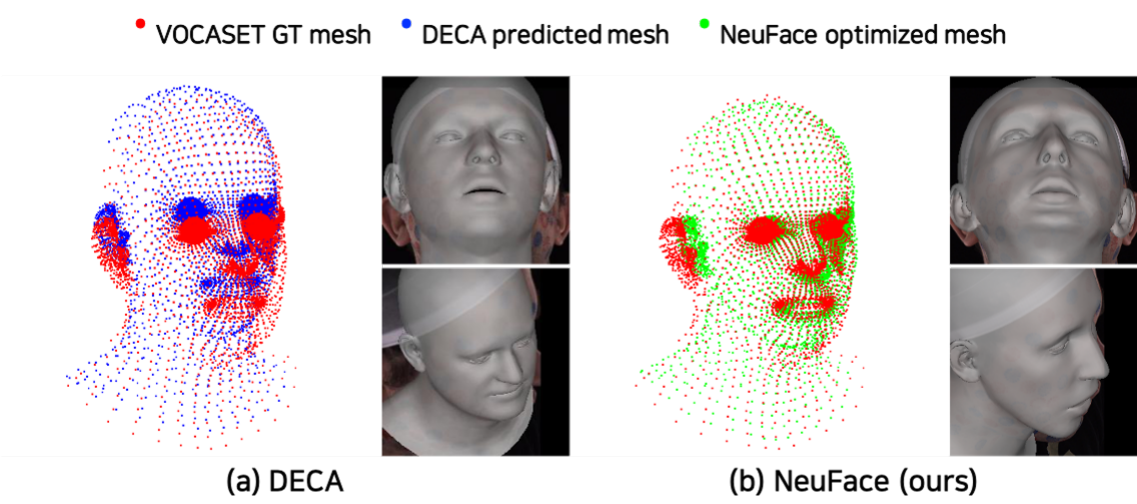}
    \vspace{3mm}
  \resizebox{1\linewidth}{!}{
  \begin{tabular}{l cccc}
  \toprule
  % &\multicolumn{2}{c}{Methods} \\
  % \cmidrule(lr){2-3} 
  Method & CVD $\downarrow$ &  MSI\textsubscript{3D, lmk} $\uparrow$\ & MSI\textsubscript{3D, vtx} $\uparrow$ & MPVE [\emph{mm}] $\downarrow$ \\
  \cmidrule(lr){1-5} 
  DECA~\citep{DECA:Siggraph2021} & 0.440 & 0.005 & 0.006 & 39.9\\
  NeuFace (ours) & \textbf{0.322}  & \textbf{0.379} &\textbf{ 0.530}& \textbf{31.2}\\
  \bottomrule
  \end{tabular}}\vspace{-3mm}
  \caption{\textbf{Accuracy of NeuFace optimization on motion capture dataset w/ GT.}
  % \kim{
  Given the ground-truth meshes of multi-view motion captured dataset, VOCASET, our NeuFace optimization reconstructs spatio-temporally consistent and more vertex-level accurate (MPVE) meshes than the off-the-shelf neural model, DECA. 
  % 
  % $\emph{Abbr.}$ lmk: landmark, vtx: vertex.
  }
%     \caption{\textbf{VOCASET result.}
%     % 
%     We visualize and compare the meshes obtained by EMOCA~\citep{EMOCA:CVPR:2022} and NeuFace.
%     % 
%     By aligning the meshes to face the same direction, we can clearly notice that
% NeuFace regresses multi-view consistent meshes compared to EMOCA.
%     }
    % \vspace{-3mm}
    \label{fig:vocaset}
\end{figure}
