# Supplementary material for: A Large-Scale 3D Face Mesh Video Dataset via Neural Re-parameterized Optimization
Source: arXiv:2310.03205 source file (2023-10-06)
Supplement: Supplementary file 4 [file supp_baseline.tex]

\begin{table*}[hbt!]
  \label{tab:quant}
  \centering
  \resizebox{\linewidth}{!}{
  \begin{tabular}{l cccc ccc ccc}
  \toprule
&\multicolumn{4}{c}{MEAD~\citep{kaisiyuan2020mead}} & \multicolumn{3}{c}{VoxCeleb2\citep{voxceleb2}} & \multicolumn{3}{c}{CelebV-HQ~\citep{zhu2022celebvhq}} \\
    \cmidrule(lr){2-5} \cmidrule(lr){6-8} \cmidrule(lr){9-11}
    \multicolumn{1}{c}{Dataset} & \multicolumn{1}{c}{CVD $\downarrow$} & \multicolumn{1}{c}{MSI\textsubscript{3D, lmk} $\uparrow$} &\multicolumn{1}{c}{MSI\textsubscript{3D, vtx} $\uparrow$} & \multicolumn{1}{c}{NME $\downarrow$} & \multicolumn{1}{c}{MSI\textsubscript{3D, lmk} $\uparrow$} &\multicolumn{1}{c}{MSI\textsubscript{3D, vtx} $\uparrow$} & \multicolumn{1}{c}{NME $\downarrow$} & \multicolumn{1}{c}{MSI\textsubscript{3D, lmk} $\uparrow$} &\multicolumn{1}{c}{MSI\textsubscript{3D, vtx} $\uparrow$} & \multicolumn{1}{c}{NME $\downarrow$} \\
  \cmidrule{1-11}
\multicolumn{1}{l}{Base-dataset}  & 0.209 & 0.011&0.016 & 4.65 & 0.028 & 0.044 & 4.78 & 0.012 & 0.018 &5.34\\
\multicolumn{1}{l}{Direct Flame opt. (Eq.~(\colorref{a}))}  & 0.192 & 0.034& 0.053 & 4.34 & 0.034 & 0.056 & 3.32 & 0.030 & 0.047 & 3.65\\
\multicolumn{1}{l}{\textbf{NeuFace-dataset (ours)}} & \textbf{0.103} & \textbf{0.206} & \textbf{0.305} & \textbf{2.58} & \textbf{0.095} & \textbf{0.137} & \textbf{2.19} & \textbf{0.054}&\textbf{0.074}&\textbf{2.55}\\
    \bottomrule
  \end{tabular}}
  % \vspace{1mm}
  % \caption{\textbf{Quantitative evaluation results.}
  % We evaluate the quantitative quality of the face meshes reconstructed with NeuFace. For sampled sequences for MEAD, VoxCeleb2 and CelebV-HQ, NeuFace reliably outperforms the competing method, DECA, for all the aspects; multi-view consistency (CVD), temporal consistency (MSI\textsubscript{3D}) and 2D landmark accuracy (NME~\citep{sagonas2016300}). $\emph{Abbr.}$ $lmk$: landmark, $vtx$: vertex.}
  \caption{\textbf{Quantitative comparison: Direct FLAME opt. vs. NeuFace.}
  % \kim{
  We evaluate the meshes obtained by the direct FLAME opt. (\Eref{eq:baseline}) and meshes in NeuFace-dataset in terms of multi-view consistency (CVD), temporal consistency (MSI\textsubscript{3D}) and the 2D landmark accuracy (NME~\citep{sagonas2016300}). 
  The results show that NeuFace-dataset significantly outperforms the meshes obtained by other solid baselines.}\vspace{-3mm}
  % }
\label{tab:baseline}
\end{table*}
