# Supplementary material for: A Large-Scale 3D Face Mesh Video Dataset via Neural Re-parameterized Optimization
Source: arXiv:2310.03205 source file (2023-10-06)
Supplement: Supplementary file 5 [file supp_emoca_quant.tex]

\begin{table*}[h!]
  \centering
  \resizebox{\linewidth}{!}{
  \begin{tabular}{l cccc ccc ccc}
  \toprule
&\multicolumn{4}{c}{MEAD~\citep{kaisiyuan2020mead}} & \multicolumn{3}{c}{VoxCeleb2\citep{voxceleb2}} & \multicolumn{3}{c}{CelebV-HQ~\citep{zhu2022celebvhq}} \\
    \cmidrule(lr){2-5} \cmidrule(lr){6-8} \cmidrule(lr){9-11}
    \multicolumn{1}{c}{Method} & \multicolumn{1}{c}{CVD $\downarrow$} & \multicolumn{1}{c}{MSI\textsubscript{3D, lmk} $\uparrow$} &\multicolumn{1}{c}{MSI\textsubscript{3D, vtx} $\uparrow$} & \multicolumn{1}{c}{NME $\downarrow$} & \multicolumn{1}{c}{MSI\textsubscript{3D, lmk} $\uparrow$} &\multicolumn{1}{c}{MSI\textsubscript{3D, vtx} $\uparrow$} & \multicolumn{1}{c}{NME $\downarrow$} & \multicolumn{1}{c}{MSI\textsubscript{3D, lmk} $\uparrow$} &\multicolumn{1}{c}{MSI\textsubscript{3D, vtx} $\uparrow$} & \multicolumn{1}{c}{NME $\downarrow$} \\
  \cmidrule{1-11}
\multicolumn{1}{l}{EMOCA~\citep{EMOCA:CVPR:2022}}  & 0.199 & 0.010 &0.016 & 5.42 & 0.003 & 0.004 & 4.77 & 0.005 & 0.007 &5.57\\
\multicolumn{1}{l}{NeuFace-E (ours)} & \textbf{0.104} & \textbf{0.209} & \textbf{0.312} & \textbf{2.28} & \textbf{0.028} & \textbf{0.048} & \textbf{2.38} & \textbf{0.053}&\textbf{0.077}&\textbf{2.86}\\
    \bottomrule
  \end{tabular}}
  % \vspace{1mm}
  % \caption{\textbf{Quantitative evaluation results.}
  % We evaluate the quantitative quality of the face meshes reconstructed with STREAM. For sampled sequences for MEAD, VoxCeleb2 and CelebV-HQ, STREAM reliably outperforms the competing method, DECA, for all the aspects; multi-view consistency (CVD), temporal consistency (MSI\textsubscript{3D}) and 2D landmark accuracy (NME~\citep{sagonas2016300}). $\emph{Abbr.}$ $lmk$: landmark, $vtx$: vertex.}
  \caption{\textbf{Quantitative comparison: EMOCA vs. NeuFace-E.}
  % \kim{
  % We optimize EMOCA with our optimization pipeline and obtain 3D faces for the validation sets. 
  We evaluate face meshes obtained using NeuFace-E and EMOCA with the metrics, CVD, MSI\textsubscript{3D}, and NME~\citep{sagonas2016300}.
  % multi-view consistency (CVD) and temporal consistency (MSI\textsubscript{3D}), along with the 2D landmark accuracy (NME~\citep{sagonas2016300}). 
  The results show that NeuFace-E significantly outperforms the competing method, EMOCA, in overall metrics. 
  % CVD and NME are measured in FLAME canonical coordinate and pixel space, respectively, while MSIs are normalized with min-max scaling.
  $\emph{Abbr.}$ lmk: landmark, vtx: vertex.
  }
  % \vspace{3mm}
  % }
\label{tab:emocaquant}
\end{table*}
